# Supplementary material for: Frequency Diverse Array-enabled RIS-aided Integrated Sensing and Communication
Source: arXiv:2410.00376 source file (2024-10-01)
Supplement: Supplementary file 1 [file SuppMaterial.pdf]

# Frequency Diverse Array-enabled RIS-aided Integrated Sensing and Communication: Supplementary Material

Hanyu Yang, Shiqi Gong, Heng Liu, Chengwen Xing, *Member, IEEE*, Nan Zhao, *Senior Member, IEEE*, and Dusit Niyato, *Fellow, IEEE*

This manuscript provides additional information for the paper titled "Frequency Diverse Array-enabled RIS-aided Integrated Sensing and Communication" by the same authors [1].

## I. Supplementary Material

Firstly, specific mathematical expressions of the cosine-form functions in problem (P3-4-1), i.e., $g_{i,k,k'}(\Delta f_{n_{\rm t}})$, $g_{j,k}(\Delta f_{n_{\rm t}})$, $g_{c,k}(\Delta f_{n_{\rm t}})$, $g_{{\rm T},k}(\Delta f_{n_{\rm t}})$, $i=$1,2,3, $j=1,2$, are derived in the following. Specifically, the function $g_{1,k,k'}(\Delta f_{n_{\rm t}})$ is reformulated from $|\alpha_k|^2|\mathbf{w}_{k'}^{\rm H}(\mathbf{g}_{{\rm BU},k}^{\rm LoS}\circ\mathbf{f}_{{\rm BU},k})|^2$ by omitting the constant irrelevant to $\Delta f_{n_{\rm t}}$, and is given by

$$\begin{aligned} g_{1,k,k'}(\Delta f_{n_{\rm t}}) =& \sum_{q\in\mathcal{N}_{\rm t}/\{n_{\rm t}\}} \underbrace{|\alpha_k|^2\left|[\mathbf{w}_{k'}]_{n_{\rm t}}^*[\mathbf{g}_{{\rm BU},k}^{\rm LoS}]_{n_{\rm t}}[\mathbf{g}_{{\rm BU},k}^{\rm LoS}]_q^*[\mathbf{w}_{k'}]_q\right|}_{\xi_{g_{1,k,k'},n_{\rm t},q}} \\ &\times\cos\Big(\underbrace{\frac{2\pi(D_{\rm BR}+D_{{\rm RU},k})}{\rm c}}_{\eta_{g_{1,k}}}\Delta f_{n_{\rm t}}\underbrace{-\frac{2\pi(D_{\rm BR}+D_{{\rm RU},k})}{\rm c}\Delta f_q+\angle([\mathbf{w}_{k'}]_{n_{\rm t}}^*[\mathbf{g}_{{\rm BU},k}^{\rm LoS}]_{n_{\rm t}}[\mathbf{g}_{{\rm BU},k}^{\rm LoS}]_q^*[\mathbf{w}_{k'}]_q)}_{\rho_{g_{1,k,k'},n_{\rm t},q}}\Big), \\ & k,k'\in\mathcal{K}, n_{\rm t}\in\mathcal{N}_{\rm t}, q\in\mathcal{N}_{\rm t}/\{n_{\rm t}\}. \end{aligned} \tag{63}$$

That is to say, $g_{1,k,k'}(\Delta f_{n_{\rm t}})$ takes the following form

$$g_{1,k,k'}(\Delta f_{n_{\rm t}})=\sum\nolimits_q \xi_{g_{1,k,k'},n_{\rm t},q}\cos(\eta_{g_{1,k}}\Delta f_{n_{\rm t}}+\rho_{g_{1,k,k'},n_{\rm t},q}). \tag{64}$$

Similarly, the remaining functions are respectively given by

$$g_{2,k,k'}(\Delta f_{n_{\rm t}}) = \sum_{q\in\mathcal{N}_{\rm t}/\{n_{\rm t}\}} \underbrace{|\alpha_k|^2\left|[\mathbf{w}_{k'}]_{n_{\rm t}}^*[\mathbf{g}_{{\rm BU},k}^{\rm NLoS}]_{n_{\rm t}}[\mathbf{g}_{{\rm BU},k}^{\rm NLoS}]_q^*[\mathbf{w}_{k'}]_q\right|}_{\xi_{g_{2,k,k'},n_{\rm t},q}}$$

$$\times\cos\Big(\underbrace{\frac{2\pi D_{\rm BR}}{\rm c}}_{\eta_{g_2}}\Delta f_{n_{\rm t}}\underbrace{-\frac{2\pi D_{\rm BR}}{\rm c}\Delta f_q+\angle([\mathbf{w}_{k'}]^*_{n_{\rm t}}[\mathbf{g}^{\rm NLoS}_{{\rm BU},k}]_{n_{\rm t}}[\mathbf{g}^{\rm NLoS}_{{\rm BU},k}]^*_q[\mathbf{w}_{k'}]_q)}_{\rho_{g_{2,k,k'},n_{\rm t},q}}\Big). \tag{65}$$

$$g_{3,k,k'}(\Delta f_{n_{\rm t}})=\sum_{q\in\mathcal{N}_{\rm t}/\{n_{\rm t}\}}\underbrace{|\alpha_k|^2\big|[\mathbf{w}_{k'}]^*_{n_{\rm t}}[\mathbf{g}^{\rm LoS}_{{\rm BU},k}]_{n_{\rm t}}[\mathbf{g}^{\rm NLoS}_{{\rm BU},k}]^*_q[\mathbf{w}_{k'}]_q\big|}_{\xi_{g_{3,k,k'},n_{\rm t},q}}$$
$$\times\cos\Big(\underbrace{\frac{2\pi(D_{\rm BR}+D_{{\rm RU},k})}{\rm c}}_{\eta_{g_{3,k}}}\Delta f_{n_{\rm t}}\underbrace{-\frac{2\pi D_{\rm BR}}{\rm c}\Delta f_q+\angle([\mathbf{w}_{k'}]^*_{n_{\rm t}}[\mathbf{g}^{\rm LoS}_{{\rm BU},k}]_{n_{\rm t}}[\mathbf{g}^{\rm NLoS}_{{\rm BU},k}]^*_q[\mathbf{w}_{k'}]_q)}_{\rho_{g_{3,k,k'},n_{\rm t},q}}\Big)$$
$$+\sum_{q\in\mathcal{N}_{\rm t}/\{n_{\rm t}\}}\underbrace{|\alpha_k|^2\big|[\mathbf{w}_{k'}]^*_q[\mathbf{g}^{\rm LoS}_{{\rm BU},k}]_q[\mathbf{g}^{\rm NLoS}_{{\rm BU},k}]^*_{n_{\rm t}}[\mathbf{w}_{k'}]_{n_{\rm t}}\big|}_{\bar{\xi}_{g_{3,k,k'},n_{\rm t},q}}$$
$$\times\cos\Big(\underbrace{\frac{2\pi D_{\rm BR}}{\rm c}}_{\bar{\eta}_{g_3}}\Delta f_{n_{\rm t}}\underbrace{-\frac{2\pi(D_{\rm BR}+D_{{\rm RU},k})}{\rm c}\Delta f_q-\angle([\mathbf{w}_{k'}]^*_q[\mathbf{g}^{\rm LoS}_{{\rm BU},k}]_q[\mathbf{g}^{\rm NLoS}_{{\rm BU},k}]^*_{n_{\rm t}}[\mathbf{w}_{k'}]_{n_{\rm t}})}_{\bar{\rho}_{g_{3,k,k'},n_{\rm t},q}}\Big)$$
$$+\underbrace{|\alpha_k|^2\big|[\mathbf{w}_{k'}]^*_{n_{\rm t}}[\mathbf{g}^{\rm LoS}_{{\rm BU},k}]_{n_{\rm t}}[\mathbf{g}^{\rm NLoS}_{{\rm BU},k}]^*_{n_{\rm t}}[\mathbf{w}_{k'}]_{n_{\rm t}}\big|}_{\acute{\xi}_{g_{3,k,k'},n_{\rm t}}}$$
$$\times\cos\Big(\underbrace{\frac{2\pi D_{{\rm RU},k}}{\rm c}}_{\acute{\eta}_{g_{3,k}}}\Delta f_{n_{\rm t}}+\underbrace{\angle([\mathbf{w}_{k'}]^*_{n_{\rm t}}[\mathbf{g}^{\rm LoS}_{{\rm BU},k}]_{n_{\rm t}}[\mathbf{g}^{\rm NLoS}_{{\rm BU},k}]^*_{n_{\rm t}}[\mathbf{w}_{k'}]_{n_{\rm t}})}_{\acute{\rho}_{g_{3,k,k'},n_{\rm t}}}\Big), \tag{66}$$

$$g_{1,k}(\Delta f_{n_{\rm t}})=\underbrace{\sqrt{1+w_k}\big|\alpha_k[\mathbf{w}_k]^*_{n_{\rm t}}[\mathbf{g}^{\rm LoS}_{{\rm BU},k}]_{n_{\rm t}}\big|}_{\xi_{g_{1,k},n_{\rm t}}}$$
$$\times\cos\Big(\underbrace{\frac{2\pi(D_{\rm BR}+D_{{\rm RU},k})}{\rm c}}_{\eta_{g_{1,k}}}\Delta f_{n_{\rm t}}+\underbrace{\angle(\alpha_k[\mathbf{w}_k]^*_{n_{\rm t}}[\mathbf{g}^{\rm LoS}_{{\rm BU},k}]_{n_{\rm t}})+\pi}_{\rho_{g_{1,k},n_{\rm t}}}\Big). \tag{67}$$

$$g_{2,k}(\Delta f_{n_{\rm t}})=\underbrace{\sqrt{1+w_k}\big|\alpha_k[\mathbf{w}_k]^*_{n_{\rm t}}[\mathbf{g}^{\rm NLoS}_{{\rm BU},k}]_{n_{\rm t}}\big|}_{\xi_{g_{2,k},n_{\rm t}}}\cos\Big(\underbrace{\frac{2\pi D_{\rm BR}}{\rm c}}_{\eta_{g_2}}\Delta f_{n_{\rm t}}+\underbrace{\angle(\alpha_k[\mathbf{w}_k]^*_{n_{\rm t}}[\mathbf{g}^{\rm NLoS}_{{\rm BU}_k}]_{n_{\rm t}})+\pi}_{\rho_{g_{2,k},n_{\rm t}}}\Big). \tag{68}$$

$$g_{c,k}(\Delta f_{n_{\rm t}})=\sum_{q\in\mathcal{N}_{\rm t}/\{n_{\rm t}\}}\underbrace{\big|[\mathbf{w}_k]^*_{n_{\rm t}}[\mathbf{g}_{{\rm BC},c}]_{n_{\rm t}}[\mathbf{g}_{{\rm BC},c}]^*_q[\mathbf{w}_k]_q\big|}_{\xi_{g_{c,k},n_{\rm t},q}}$$
$$\times\cos\Big(\underbrace{\frac{2\pi(D_{\rm BR}+D_{{\rm RC},c})}{\rm c}}_{\eta_{g_c}}\Delta f_{n_{\rm t}}\underbrace{-\frac{2\pi(D_{\rm BR}+D_{{\rm RC},c})}{\rm c}\Delta f_q+\angle([\mathbf{w}_k]^*_{n_{\rm t}}[\mathbf{g}_{{\rm BC},c}]_{n_{\rm t}}[\mathbf{g}_{{\rm BC},c}]^*_q[\mathbf{w}_k]_q)}_{\rho_{g_{c,k},n_{\rm t},q}}\Big). \tag{69}$$

$$g_{{\rm T},k}(\Delta f_{n_{\rm t}})=\sum_{q\in\mathcal{N}_{\rm t}/\{n_{\rm t}\}}\underbrace{\big|[\mathbf{w}_k]^*_{n_{\rm t}}[\mathbf{g}_{\rm BT}]_{n_{\rm t}}[\mathbf{g}_{\rm BT}]^*_q[\mathbf{w}_k]_q\big|}_{\xi_{g_{{\rm T},k},n_{\rm t},q}}$$

$$\times \cos\big(\underbrace{\frac{2\pi(D_{\rm BR}+D_{\rm RT})}{\rm c}}_{\eta_{\rm T}}\Delta f_{n_{\rm t}} \underbrace{-\frac{2\pi(D_{\rm BR}+D_{\rm RT})}{\rm c}\Delta f_q+\angle([\mathbf{w}_k]^*_{n_{\rm t}}[\mathbf{g}_{\rm BT}]_{n_{\rm t}}[\mathbf{g}_{\rm BT}]^*_q[\mathbf{w}_k]_q)+\pi}_{\rho_{g_{{\rm T},k},n_{\rm t},q}}\big). \tag{70}$$

It follows from (63)-(70) that the specific values of $\{\xi_l,\eta_l,\rho_l\}$ with $l$ representing the summation index associated with different functions $g_{i,k,k'}(\Delta f_{n_{\rm t}})$,$g_{j,k}(\Delta f_{n_{\rm t}})$,$g_{c,k}(\Delta f_{n_{\rm t}})$,$g_{{\rm T},k}(\Delta f_{n_{\rm t}})$, $i=$ 1,2,3, $j=1,2$ are respectively given by

$$\begin{aligned}&\{\xi_l,\eta_l,\rho_l\}\triangleq\{\xi_{g_{1,k,k'},n_{\rm t},q},\eta_{g_{1,k}},\rho_{g_{1,k,k'},n_{\rm t},q}\},\{\xi_{g_{2,k,k'},n_{\rm t},q},\eta_{g_2},\rho_{g_{2,k,k'},n_{\rm t},q}\},\\&\{\xi_{g_{3,k,k'},n_{\rm t},q},\eta_{g_{3,k}},\rho_{g_{3,k,k'},n_{\rm t},q},\overline{\xi}_{g_{3,k,k'},n_{\rm t},q},\overline{\eta}_{g_3},\overline{\rho}_{g_{3,k,k'},n_{\rm t},q},\acute{\xi}_{g_{3,k,k'},n_{\rm t}},\acute{\eta}_{g_{3,k}},\acute{\rho}_{g_{3,k,k'},n_{\rm t}}\},\\&\{\xi_{g_{1,k},n_{\rm t}},\eta_{g_{1,k}},\rho_{g_{1,k},n_{\rm t}}\},\{\xi_{g_{2,k},n_{\rm t}},\eta_{g_2},\rho_{g_{2,k},n_{\rm t}}\},\{\xi_{g_{c,k},n_{\rm t},q},\eta_{g_c},\rho_{g_{c,k},n_{\rm t},q}\},\{\xi_{g_{{\rm T},k},n_{\rm t},q},\eta_{\rm T},\rho_{g_{{\rm T},k},n_{\rm t},q}\},\\&k,k'\in\mathcal{K},n_{\rm t}\in\mathcal{N}_{\rm t},q\in\mathcal{N}_{\rm t}/\{n_{\rm t}\},c\in\mathcal{C}.\end{aligned}$$

Moreover, the constant $\gamma_{\rm T}^{\rm cons}$ irrelevant to $\Delta f_{n_{\rm t}}$ in the SCNR constraint in problem (P3-4-1) is given by

$$\begin{aligned}\gamma_{\rm T}^{\rm cons}=&\sum\nolimits_{k\in\mathcal{K},p,q\in\mathcal{N}_{\rm t}/\{n_{\rm t}\}}\big(\sum\nolimits_{c=1}^{C}\gamma_{\rm T}[\mathbf{w}_k]^*_p[\mathbf{g}_{{\rm BC},c}]_p[\mathbf{g}_{{\rm BC},c}]^*_q[\mathbf{w}_k]_q-[\mathbf{w}_k]^*_p[\mathbf{g}_{\rm BT}]_p[\mathbf{g}_{\rm BT}]^*_q[\mathbf{w}_k]_q\big)\\&+\sum\nolimits_{k=1}^{K}\big(\sum\nolimits_{c=1}^{C}\gamma_{\rm T}\big|[\mathbf{w}_k]^*_{n_{\rm t}}[\mathbf{g}_{{\rm BC},c}]_{n_{\rm t}}\big|^2-\big|[\mathbf{w}_k]^*_{n_{\rm t}}[\mathbf{g}_{\rm BT}]_{n_{\rm t}}\big|^2\big)+\gamma_{\rm T}\|\mathbf{u}\|^2\sigma_{\rm R}^2.\end{aligned} \tag{71}$$

Hereafter, we aim to derive the specific mathematical expressions of the convex quadratic functions $\hat{g}_{i,k,k'}(\Delta f_{n_{\rm t}})$, $\hat{g}_{j,k}(\Delta f_{n_{\rm t}})$, $\hat{g}_{c,k}(\Delta f_{n_{\rm t}})$, $\hat{g}_{{\rm T},k}(\Delta f_{n_{\rm t}})$, $i=1,2,3,j=1,2$ in problem (P3-4-2). Specifically, $\hat{g}_{1,k,k'}(\Delta f_{n_{\rm t}})$ is given by

$$\hat{g}_{1,k,k'}(\Delta f_{n_{\rm t}})=\sum\nolimits_q\big(\hat{\xi}^{(j)}_{g_{1,k,k'},n_{\rm t},q}(\Delta f_{n_{\rm t}}-\hat{\eta}^{(j)}_{g_{1,k,k'},n_{\rm t},q})^2+\hat{\rho}^{(j)}_{g_{1,k,k'},n_{\rm t},q}\big),k,k'\in\mathcal{K},n_{\rm t}\in\mathcal{N}_{\rm t},q\in\mathcal{N}_{\rm t}/\{n_{\rm t}\}, \tag{72}$$

where $\{\hat{\xi}^{(j)}_{g_{1,k,k'},n_{\rm t},q},\hat{\eta}^{(j)}_{g_{1,k,k'},n_{\rm t},q},\hat{\rho}^{(j)}_{g_{1,k,k'},n_{\rm t},q}\}$ are derived according to the following two cases by referring to [2].

**Case 1.** $\sin(\eta_{g_{1,k}}\Delta f^{(j)}_{n_{\rm t}}+\rho_{g_{1,k,k'},n_{\rm t},q})\neq 0$:

$$\hat{\xi}^{(j)}_{g_{1,k,k'},n_{\rm t},q}=-\frac{\xi_{g_{1,k,k'},n_{\rm t},q}\eta_{g_{1,k}}\sin(\eta_{g_{1,k}}\Delta f^{(j)}_{n_{\rm t}}+\rho_{g_{1,k,k'},n_{\rm t},q})}{2(\Delta f^{(j)}_{n_{\rm t}}-\hat{\eta}^{(j)}_{g_{1,k,k'},n_{\rm t},q})},$$

$$\hat{\eta}^{(j)}_{g_{1,k,k'},n_{\rm t},q}=\begin{cases}\pi\dfrac{\Big\lfloor\Big(\frac{\eta_{g_{1,k}}\Delta f^{(j)}_{n_{\rm t}}}{\pi}+\frac{\rho_{g_{1,k,k'},n_{\rm t},q}}{\pi}\Big)\Big\rfloor-\frac{\rho_{g_{1,k,k'},n_{\rm t},q}}{\pi}}{\eta_{g_{1,k}}}, & \sin(\eta_{g_{1,k}}\Delta f^{(j)}_{n_{\rm t}}+\rho_{g_{1,k,k'},n_{\rm t},q})<0\\ \pi\dfrac{\Big\lceil\Big(\frac{\eta_{g_{1,k}}\Delta f^{(j)}_{n_{\rm t}}}{\pi}+\frac{\rho_{g_{1,k,k'},n_{\rm t},q}}{\pi}\Big)\Big\rceil-\frac{\rho_{g_{1,k,k'},n_{\rm t},q}}{\pi}}{\eta_{g_{1,k}}}, & \text{otherwise}\end{cases},$$

$$\hat{\rho}^{(j)}_{g_{1,k,k'},n_{\mathrm{t}},q}=\xi_{g_{1,k,k'},n_{\mathrm{t}},q}\big(\cos(\eta_{g_{1,k}}\Delta f^{(j)}_{n_{\mathrm{t}}}+\rho_{g_{1,k,k'},n_{\mathrm{t}},q})-\hat{\xi}^{(j)}_{g_{1,k,k'},n_{\mathrm{t}},q}(\Delta f^{(j)}_{n_{\mathrm{t}}}-\hat{\eta}^{(j)}_{g_{1,k,k'},n_{\mathrm{t}},q})^2\big). \tag{73}$$

**Case 2.** $\sin(\eta_{g_{1,k}}\Delta f^{(j)}_{n_{\mathrm{t}}}+\rho_{g_{1,k,k'},n_{\mathrm{t}},q})=0$:

$$\hat{\xi}^{(j)}_{g_{1,k,k'},n_{\mathrm{t}},q}=\begin{cases}0, & \cos(\eta_{g_{1,k}}\Delta f^{(j)}_{n_{\mathrm{t}}}+\rho_{g_{1,k,k'},n_{\mathrm{t}},q})=1\\ \xi_{g_{1,k,k'},n_{\mathrm{t}},q}2\pi^2(\Delta f^{(j)}_{n_{\mathrm{t}}})^2, & \text{otherwise}\end{cases},$$

$$\hat{\eta}^{(j)}_{g_{1,k,k'},n_{\mathrm{t}},q}=\Delta f^{(j)}_{n_{\mathrm{t}}},\hat{\rho}^{(j)}_{g_{1,k,k'},n_{\mathrm{t}},q}=\xi_{g_{1,k,k'},n_{\mathrm{t}},q}\cos(\eta_{g_{1,k}}\Delta f^{(j)}_{n_{\mathrm{t}}}+\rho_{g_{1,k,k'},n_{\mathrm{t}},q}). \tag{74}$$

In particular, in (73) and (74), $\Delta f^{(j)}_{n_{\mathrm{t}}}$ denotes the $j$-th SCA iteration point. Moreover, the remaining functions $\hat{g}_{i,k,k'}(\Delta f_{n_{\mathrm{t}}})$, $\hat{g}_{j,k}(\Delta f_{n_{\mathrm{t}}})$, $\hat{g}_{c,k}(\Delta f_{n_{\mathrm{t}}})$, $\hat{g}_{\mathrm{T},k}(\Delta f_{n_{\mathrm{t}}})$, $i=2,3, j=1,2$ are respectively given by

$$\hat{g}_{2,k,k'}(\Delta f_{n_{\mathrm{t}}})=\sum\nolimits_q\big(\hat{\xi}^{(j)}_{g_{2,k,k'},n_{\mathrm{t}},q}(\Delta f_{n_{\mathrm{t}}}-\hat{\eta}^{(j)}_{g_{2,k,k'},n_{\mathrm{t}},q})^2+\hat{\rho}^{(j)}_{g_{2,k,k'},n_{\mathrm{t}},q}\big), \tag{75}$$

$$\begin{aligned}\hat{g}_{3,k,k'}(\Delta f_{n_{\mathrm{t}}})=&\sum\nolimits_q\big(\hat{\xi}^{(j)}_{g_{3,k,k'},n_{\mathrm{t}},q}(\Delta f_{n_{\mathrm{t}}}-\hat{\eta}^{(j)}_{g_{3,k,k'},n_{\mathrm{t}},q})^2+\hat{\rho}^{(j)}_{g_{3,k,k'},n_{\mathrm{t}},q}\big)\\ &+\sum\nolimits_q\big(\tilde{\xi}^{(j)}_{g_{3,k,k'},n_{\mathrm{t}},q}(\Delta f_{n_{\mathrm{t}}}-\tilde{\eta}^{(j)}_{g_{3,k,k'},n_{\mathrm{t}},q})^2+\tilde{\rho}^{(j)}_{g_{3,k,k'},n_{\mathrm{t}},q}\big)\\ &+\grave{\xi}^{(j)}_{g_{3,k,k'},n_{\mathrm{t}}}(\Delta f_{n_{\mathrm{t}}}-\grave{\eta}^{(j)}_{g_{3,k,k'},n_{\mathrm{t}}})^2+\grave{\rho}^{(j)}_{g_{3,k,k'},n_{\mathrm{t}}},\end{aligned} \tag{76}$$

$$\hat{g}_{1,k}(\Delta f_{n_{\mathrm{t}}})=\hat{\xi}^{(j)}_{g_{1,k},n_{\mathrm{t}}}(\Delta f_{n_{\mathrm{t}}}-\hat{\eta}^{(j)}_{g_{1,k},n_{\mathrm{t}}})^2+\hat{\rho}^{(j)}_{g_{1,k},n_{\mathrm{t}}}, \tag{77}$$

$$\hat{g}_{2,k}(\Delta f_{n_{\mathrm{t}}})=\hat{\xi}^{(j)}_{g_{2,k},n_{\mathrm{t}}}(\Delta f_{n_{\mathrm{t}}}-\hat{\eta}^{(j)}_{g_{2,k},n_{\mathrm{t}}})^2+\hat{\rho}^{(j)}_{g_{2,k},n_{\mathrm{t}}}, \tag{78}$$

$$\hat{g}_{c,k}(\Delta f_{n_{\mathrm{t}}})=\sum\nolimits_q\big(\hat{\xi}^{(j)}_{g_{c,k},n_{\mathrm{t}},q}(\Delta f_{n_{\mathrm{t}}}-\hat{\eta}^{(j)}_{g_{c,k},n_{\mathrm{t}},q})^2+\hat{\rho}^{(j)}_{g_{c,k},n_{\mathrm{t}},q}\big), \tag{79}$$

$$\hat{g}_{\mathrm{T},k}(\Delta f_{n_{\mathrm{t}}})=\sum\nolimits_q\big(\hat{\xi}^{(j)}_{g_{\mathrm{T},k},n_{\mathrm{t}},q}(\Delta f_{n_{\mathrm{t}}}-\hat{\eta}^{(j)}_{g_{\mathrm{T},k},n_{\mathrm{t}},q})^2+\hat{\rho}^{(j)}_{g_{\mathrm{T},k},n_{\mathrm{t}},q}\big), \tag{80}$$

where the specific values of

$$\begin{aligned}&\{\hat{\xi}^{(j)}_{g_{2,k,k'},n_{\mathrm{t}},q},\hat{\eta}^{(j)}_{g_{2,k,k'},n_{\mathrm{t}},q},\hat{\rho}^{(j)}_{g_{2,k,k'},n_{\mathrm{t}},q}\},\\ &\{\hat{\xi}^{(j)}_{g_{3,k,k'},n_{\mathrm{t}},q},\hat{\eta}^{(j)}_{g_{3,k,k'},n_{\mathrm{t}},q},\hat{\rho}^{(j)}_{g_{3,k,k'},n_{\mathrm{t}},q},\tilde{\xi}^{(j)}_{g_{3,k,k'},n_{\mathrm{t}},q},\tilde{\eta}^{(j)}_{g_{3,k,k'},n_{\mathrm{t}},q},\tilde{\rho}^{(j)}_{g_{3,k,k'},n_{\mathrm{t}},q},\grave{\xi}^{(j)}_{g_{3,k,k'},n_{\mathrm{t}}},\grave{\eta}^{(j)}_{g_{3,k,k'},n_{\mathrm{t}}},\grave{\rho}^{(j)}_{g_{3,k,k'},n_{\mathrm{t}}}\},\\ &\{\hat{\xi}^{(j)}_{g_{1,k},n_{\mathrm{t}}},\hat{\eta}^{(j)}_{g_{1,k},n_{\mathrm{t}}},\hat{\rho}^{(j)}_{g_{1,k},n_{\mathrm{t}}}\},\{\hat{\xi}^{(j)}_{g_{2,k},n_{\mathrm{t}}},\hat{\eta}^{(j)}_{g_{2,k},n_{\mathrm{t}}},\hat{\rho}^{(j)}_{g_{2,k},n_{\mathrm{t}}}\},\{\hat{\xi}^{(j)}_{g_{c,k},n_{\mathrm{t}},q},\hat{\eta}^{(j)}_{g_{c,k},n_{\mathrm{t}},q},\hat{\rho}^{(j)}_{g_{c,k},n_{\mathrm{t}},q}\},\\ &\{\hat{\xi}^{(j)}_{g_{\mathrm{T},k},n_{\mathrm{t}},q},\hat{\eta}^{(j)}_{g_{\mathrm{T},k},n_{\mathrm{t}},q},\hat{\rho}^{(j)}_{g_{\mathrm{T},k},n_{\mathrm{t}},q}\},k,k'\in\mathcal{K},n_{\mathrm{t}}\in\mathcal{N}_{\mathrm{t}},q\in\mathcal{N}_{\mathrm{t}}/\{n_{\mathrm{t}}\},c\in\mathcal{C},\end{aligned} \tag{81}$$

are derived similarly to $\{\hat{\xi}^{(j)}_{g_{1,k,k'},n_{\mathrm{t}},q},\hat{\eta}^{(j)}_{g_{1,k,k'},n_{\mathrm{t}},q},\hat{\rho}^{(j)}_{g_{1,k,k'},n_{\mathrm{t}},q}\}$

Based on (81), the objective function of problem (P3-4-2) can be equivalently rewritten as

$$\hat{f}_{\mathrm{obj}}(\Delta f_{n_{\mathrm{t}}})=\hat{d}_1\Delta f^2_{n_{\mathrm{t}}}+\hat{d}_2\Delta f_{n_{\mathrm{t}}}+\hat{d}_3 \tag{82}$$

where $\{\hat{d}_1, \hat{d}_2, \hat{d}_3\}$ are given by

$$
\begin{aligned}
\hat{d}_1 = & \sum_{k,k',q} \big( \hat{\xi}^{(j)}_{g_{1,k,k'},n_{\mathrm{t}},q} + \hat{\xi}^{(j)}_{g_{2,k,k'},n_{\mathrm{t}},q} + \hat{\xi}^{(j)}_{g_{3,k,k'},n_{\mathrm{t}},q} + \tilde{\xi}^{(j)}_{g_{3,k,k'},n_{\mathrm{t}},q} \big) + \sum_{k,k'} \grave{\xi}^{(j)}_{g_{3,k,k'},n_{\mathrm{t}}} + \sum_{k} \big( \hat{\xi}^{(j)}_{g_{1,k},n_{\mathrm{t}}} + \hat{\xi}^{(j)}_{g_{2,k},n_{\mathrm{t}}} \big), \\
\hat{d}_2 = & -2 \Big( \sum_{k,k',q} \big( \hat{\xi}^{(j)}_{g_{1,k,k'},n_{\mathrm{t}},q} \hat{\eta}^{(j)}_{g_{1,k,k'},n_{\mathrm{t}},q} + \hat{\xi}^{(j)}_{g_{2,k,k'},n_{\mathrm{t}},q} \hat{\eta}^{(j)}_{g_{2,k,k'},n_{\mathrm{t}},q} + \hat{\xi}^{(j)}_{g_{3,k,k'},n_{\mathrm{t}},q} \hat{\eta}^{(j)}_{g_{3,k,k'},n_{\mathrm{t}},q} \\
& + \tilde{\xi}^{(j)}_{g_{3,k,k'},n_{\mathrm{t}},q} \tilde{\eta}^{(j)}_{g_{3,k,k'},n_{\mathrm{t}},q} \big) + \sum_{k,k'} \grave{\xi}^{(j)}_{g_{3,k,k'},n_{\mathrm{t}}} \grave{\eta}^{(j)}_{g_{3,k,k'},n_{\mathrm{t}}} + \sum_{k} \big( \hat{\xi}^{(j)}_{g_{1,k},n_{\mathrm{t}}} \hat{\eta}^{(j)}_{g_{1,k},n_{\mathrm{t}}} + \hat{\xi}^{(j)}_{g_{2,k},n_{\mathrm{t}}} \hat{\eta}^{(j)}_{g_{2,k},n_{\mathrm{t}}} \big) \Big), \\
\hat{d}_3 = & \sum_{k,k',q} \big( \hat{\xi}^{(j)}_{g_{1,k,k'},n_{\mathrm{t}},q} (\hat{\eta}^{(j)}_{g_{1,k,k'},n_{\mathrm{t}},q})^2 + \hat{\xi}^{(j)}_{g_{2,k,k'},n_{\mathrm{t}},q} (\hat{\eta}^{(j)}_{g_{2,k,k'},n_{\mathrm{t}},q})^2 + \hat{\xi}^{(j)}_{g_{3,k,k'},n_{\mathrm{t}},q} (\hat{\eta}^{(j)}_{g_{3,k,k'},n_{\mathrm{t}},q})^2 \\
& + \tilde{\xi}^{(j)}_{g_{3,k,k'},n_{\mathrm{t}},q} (\tilde{\eta}^{(j)}_{g_{3,k,k'},n_{\mathrm{t}},q})^2 \big) + \sum_{k,k'} \grave{\xi}^{(j)}_{g_{3,k,k'},n_{\mathrm{t}}} (\grave{\eta}^{(j)}_{g_{3,k,k'},n_{\mathrm{t}}})^2 + \sum_{k} \big( \hat{\xi}^{(j)}_{g_{1,k},n_{\mathrm{t}}} (\hat{\eta}^{(j)}_{g_{1,k},n_{\mathrm{t}}})^2 + \hat{\xi}^{(j)}_{g_{2,k},n_{\mathrm{t}}} (\hat{\eta}^{(j)}_{g_{2,k},n_{\mathrm{t}}})^2 \big) \\
& + \sum_{k,k',q} \big( \hat{\rho}^{(j)}_{g_{1,k,k'},n_{\mathrm{t}},q} + \hat{\rho}^{(j)}_{g_{2,k,k'},n_{\mathrm{t}},q} + \hat{\rho}^{(j)}_{g_{3,k,k'},n_{\mathrm{t}},q} + \tilde{\rho}^{(j)}_{g_{3,k,k'},n_{\mathrm{t}},q} \big) + \sum_{k,k'} \grave{\rho}^{(j)}_{g_{3,k,k'},n_{\mathrm{t}}} + \sum_{k} \big( \hat{\rho}^{(j)}_{g_{1,k},n_{\mathrm{t}}} + \hat{\rho}^{(j)}_{g_{2,k},n_{\mathrm{t}}} \big).
\end{aligned} \tag{83}
$$

Similarly, the SCNR constraint in problem (P3-4-2) can be equivalently rewritten as

$$
\tilde{d}_1 \Delta f_{n_{\mathrm{t}}}^2 + \tilde{d}_2 \Delta f_{n_{\mathrm{t}}} + \tilde{d}_3 \leq 0, \tag{84}
$$

where $\{\tilde{d}_1, \tilde{d}_2, \tilde{d}_3\}$ are given by

$$
\begin{aligned}
\tilde{d}_1 = & \sum_{c,k,q} \hat{\xi}^{(j)}_{g_{c,k},n_{\mathrm{t}},q} + \sum_{k,q} \hat{\xi}^{(j)}_{g_{\mathrm{T},k},n_{\mathrm{t}},q}, \\
\tilde{d}_2 = & -2 \Big( \sum_{c,k,q} \hat{\xi}^{(j)}_{g_{c,k},n_{\mathrm{t}},q} \hat{\eta}^{(j)}_{g_{c,k},n_{\mathrm{t}},q} + \sum_{k,q} \hat{\xi}^{(j)}_{g_{\mathrm{T},k},n_{\mathrm{t}},q} \hat{\eta}^{(j)}_{g_{\mathrm{T},k},n_{\mathrm{t}},q} \Big), \\
\tilde{d}_3 = & \sum_{c,k,q} \hat{\xi}^{(j)}_{g_{c,k},n_{\mathrm{t}},q} (\hat{\eta}^{(j)}_{g_{c,k},n_{\mathrm{t}},q})^2 + \sum_{k,q} \hat{\xi}^{(j)}_{g_{\mathrm{T},k},n_{\mathrm{t}},q} (\hat{\eta}^{(j)}_{g_{\mathrm{T},k},n_{\mathrm{t}},q})^2 + \sum_{c,k,q} \hat{\rho}^{(j)}_{g_{c,k},n_{\mathrm{t}},q} + \sum_{k,q} \hat{\rho}^{(j)}_{g_{\mathrm{T},k},n_{\mathrm{t}},q} + \gamma_{\mathrm{T}}^{\mathrm{cons}}.
\end{aligned} \tag{85}
$$

## References


[1] H. Yang, S. Gong, H. Liu, C. Xing, N. Zhao, and D. Niyato, "Frequency diverse array-enabled RIS-aided integrated sensing and communication", *arxiv: TODO*, 2024.

[2] Y. Zhang, Y. Zhang, J. Wang, S. Xiao, and W. Tang, "Distance-angle beamforming for covert communications via frequency diverse array: Toward two-dimensional covertness," *IEEE Trans. Wireless Commun.,* vol. 22, no. 12, pp. 8559–8574, Dec. 2023.
